# Supplementary material for: $\mu$DARTS: Model Uncertainty-Aware Differentiable Architecture Search
Source: arXiv:2107.11500 source file (2022-09-11)
Supplement: Supplementary file 1 [file Appendix2.tex]

\section*{Appendix A}

\subsection*{Comparison of spectral radius of DARTS vs UDARTS}

\textbf{Proof: }
\subsubsection{High-level Proof}
The entire proof is divided into four major steps: 
\begin{itemize}
    \item We prove that the Hessian of the softmax cost is convex in nature by showing that the smallest possible eigenvalue of the Hessian of the cost function of standard DARTS is 0. 
    \begin{itemize}
        \item We do this by showing the smallest value taken by $\mathbf{z}^{T} \nabla_{\alpha}^{2} \mathcal{L}_{\text{valid}}^{\text{DARTS}} \mathbf{z}$
for any unit-length vector $\mathbf{z}$ and any possible weight vector $\mathbf{\alpha}$
\item \[\mathbf{z}^{T} \nabla_{\alpha}^{2} \mathcal{L}_{\text{valid}}^{\text{DARTS}} \mathbf{z} =\frac{1}{N} \sum_{i=1}^{N} \sigma_{i}\left(\mathbf{z}^{T} \mathbf{x}_{i}\right)^{2}\]
\item Since it is always the case that $\left(\mathbf{z}^{T} \mathbf{x}_{i}\right)^{2} \geq 0$ and $\sigma_{i} \geq 0,$ it follows that the smallest value the above can take is 0
    \end{itemize}

    \item Building on the proof, we find the largest  eigenvalue of the standard DARTS by calculating the largest value the Rayleigh quotient
    
    \item Similarly, we calculate the Hessian of the loss function of the UDARTS method which has the additional predictive variance term.
    \item We show that the largest value of the Rayleigh quotient for the UDARTS method is smaller than that of the DARTS method.
\end{itemize}

We aim to prove that the inclusion of the predictive variance improves the performance of the UDARTS method compared to normal DARTS and will search for a flatter minima.
In order to prove this, we aim to show that the spectral radius of the Hessian of the validation loss $\rho(\nabla_{\alpha}^2 \mathcal{L}_{\text{valid}})$ is smaller than the spectral radius of the normal DARTS method.  First of all we consider the cross entropy loss which is used to calculate the basic validation loss $\mathcal{L}_{\text{valid}}$. 
If $\mathbf{y}_i$ is the vector denoting the labels of the classes, $\mathbf{x}_{i}$ is the input vector and $\alpha$ is the weight matrix , the gradient and the corresponding hessian of the cross entropy loss are given as follows:
\begin{equation}\mathcal{L}_{\text{valid}}^{\text{DARTS}}=-\frac{1}{N} \sum_{i=1}^{N} \mathbf{y}_{i} \log \left(\sigma\left(\texttt{model}\left(\mathbf{x}_{i}, \mathbf{\alpha}\right)\right)\right)+\left(1-\mathbf{y}_{i}\right) \log \left(1-\sigma\left(\texttt{model}\left(\mathbf{x}_{i}, \mathbf{\alpha}\right)\right)\right)\end{equation}

For this proof we consider a linear model given as $\texttt{model}\left(\mathbf{x}_{i}, \mathbf{\alpha}\right)=\mathbf{x}_{i}^{T} \mathbf{\alpha}$

\begin{equation}\nabla_{\alpha} \mathcal{L}_{\text{valid}}^{\text{DARTS}}=-\frac{1}{N} \sum_{i=1}^{N}\left(\mathbf{y}_{i}-\sigma\left(\mathbf{x}_{i}^{T} \mathbf{\alpha}\right)\right) \mathbf{x}_{i}\end{equation}

\begin{equation}\nabla_{\alpha}^{2} \mathcal{L}_{\text{valid}}^{\text{DARTS}}=\frac{1}{N} \sum_{i=1}^{N} \sigma\left(\mathbf{x}_{i}^{T} \mathbf{\alpha}\right)\left(1-\sigma\left(\mathbf{x}_{i}^{T} \mathbf{\alpha}\right)\right) \mathbf{x}_{i} \mathbf{x}_{i}^{T}\end{equation}

Now, in order to prove that the cross entropy function is convex, we prove that the hessian is positive semi-definite. We know that the smallest eigenvalue of any square symmetric matrix is given as the minimum of the Rayleigh quotient, i.e., the smallest value taken by $\mathbf{z}^{T} \nabla_{\alpha}^{2} \mathcal{L}_{\text{valid}}^{\text{DARTS}} \mathbf{z}$
for any unit-length vector $\mathbf{z}$ and any possible weight vector $\mathbf{\alpha}$. Substituting in the particular form of the Hessian here, denoting $\sigma_{i}=\sigma\left(\mathbf{x}_{i}^{T} \mathbf{\alpha}\right)\left(1-\sigma\left(\mathbf{x}_{i}^{T} \mathbf{\alpha}\right)\right)$ for each $i$ for short, we have
\begin{equation}
\mathbf{z}^{T} \nabla_{\alpha}^{2} \mathcal{L}_{\text{valid}}^{\text{DARTS}} \mathbf{z}=\mathbf{z}^{T}\left(\frac{1}{N} \sum_{i=1}^{N} \sigma_{i} \mathbf{x}_{i} \mathbf{x}_{i}^{T}\right) \mathbf{z}=\frac{1}{N} \sum_{i=1}^{N} \sigma_{i}\left(\mathbf{z}^{T} \mathbf{x}_{i}\right)\left(\mathbf{x}_{i}^{T} \mathbf{z}\right)=\frac{1}{N} \sum_{i=1}^{N} \sigma_{i}\left(\mathbf{z}^{T} \mathbf{x}_{i}\right)^{2}
\end{equation}
Since it is always the case that $\left(\mathbf{z}^{T} \mathbf{x}_{i}\right)^{2} \geq 0$ and $\sigma_{i} \geq 0,$ it follows that the smallest value the above can take is 0 meaning that this is the smallest possible eigenvalue of the Hessian of the cost function of softmax. Since this is the case, the softmax
cost must be convex.
We know that for a matrix $A$, 
\begin{equation}\|A\|_{2}^{2}=\max _{x \neq 0} \frac{\|A x\|_{2}^{2}}{\|x\|_{2}^{2}}=\max _{x \neq 0} \frac{x^{T} A^{T} A x}{x^{T} x}=\lambda_{\max }\left(A^{T} A\right)=\rho\left(A^{T} A\right)\end{equation}

Building on the analysis above showing that the cross-entropy cost is convex, we can likewise compute its largest possible eigenvalue.% by noting that $\sigma_{i} \le \frac{1}{4}$. 
Thus the largest value the Rayleigh quotient can take is bounded above for any $\mathbf{z}$ as
\begin{equation}
    \mathbf{z}^{T} \nabla_{\alpha}^{2} \mathcal{L}_{\text{valid}}^{\text{DARTS}} \mathbf{z} \leq \frac{\max \sigma_i}{ N} \mathbf{z}^{T}\left(\sum_{i=1}^{N} \mathbf{x}_{i} \mathbf{x}_{i}^{T}\right) \mathbf{z}
\end{equation}

Since the maximum value $\mathbf{z}^{T}\left(\sum_{i=1}^{N} \mathbf{x}_{i} \mathbf{x}_{i}^{T}\right) \mathbf{z}$ can take is the maximum eigenvalue of the matrix $\sum_{i=1}^{N} \mathbf{x}_{i} \mathbf{x}_{i}^{T},$ thus the spectral radius for the Cross Entropy cost is given as
\begin{equation}
\rho(\nabla_{\alpha}^{2}\mathcal{L}_{\text{valid}}^{\text{DARTS}}) = \frac{\max \sigma_i}{N}\left\|\sum_{i=1}^{N} \mathbf{x}_{i} \mathbf{x}_{i}^{T}\right\|_{2}^{2}
\end{equation}

Now for the case of UDARTS, we add the predictive variance term to the DARTS validation loss. 
If we consider that $\sigma(\mathbf{\alpha} \mathbf{x}_{i} \mathbf{x}_{i}^{T} \mathbf{\alpha}^{T}) \rightarrow \sigma_{x^2}$ and $\sigma(\mathbf{x}_{i}^{T} \mathbf{\alpha}) \rightarrow \sigma_{x}$

\begin{align}
\operatorname{Var}_{p(\mathbf{y} | \mathbf{x})}^{model}(\mathbf{\alpha}) &= \mathbb{E}((\mathbf{x}_{i}^{T}\alpha)^2)  - \mathbb{E}(\mathbf{x}^{T}_{i}\alpha)^2
= \frac{1}{T} \sum_{i=1}^{T}\sigma( \mathbf{\alpha} \mathbf{x}_{i} \mathbf{x}_{i}^{T} \mathbf{\alpha}^{T}) - (\frac{1}{T} \sum_{i=1}^{T}\sigma(\mathbf{x}_{i}^{T} \mathbf{\alpha}))^{2} = \\
\nabla_{\alpha} \operatorname{Var}_{p(\mathbf{y} | \mathbf{x})}^{model}(\mathbf{\alpha}) 
%&= \frac{1}{T} \sum_{i=1}^{T}\sigma(\mathbf{\alpha} \mathbf{x}_{i} \mathbf{x}_{i}^{T} \mathbf{\alpha}^{T})(1- \sigma(\mathbf{\alpha} \mathbf{x}_{i} \mathbf{x}_{i}^{T} \mathbf{\alpha}^{T})) 2\mathbf{\alpha}^{T}\mathbf{x}_{i} -  \frac{2}{T^{2}} \sum_{i=1}^{T} \sigma(\mathbf{x}_{i}^{T} \mathbf{\alpha}) \sum_{i=1}^{T} \sigma(\mathbf{x}_{i}^{T} \mathbf{\alpha}) (1 - \sigma(\mathbf{x}_{i}^{T} \mathbf{\alpha})) \mathbf{x}_{i}\\
 &= \frac{1}{T} \sum_{i=1}^{T}\sigma_{x^2}(1- \sigma_{x^2}) 2\mathbf{\alpha}^{T}\mathbf{x}_{i} -  \frac{2}{T^{2}} \sum_{i=1}^{T} \sigma_{x} \sum_{i=1}^{T} \sigma_{x} (1 - \sigma_{x}) \mathbf{x}_{i} \\
\nabla_{\alpha}^{2} \operatorname{Var}_{p(\mathbf{y} | \mathbf{x})}^{model}(\mathbf{\alpha}) 
%&= \frac{1}{T} \sum_{i=1}^{T} \{ [\sigma( \mathbf{\alpha} \mathbf{x}_{i} \mathbf{x}_{i}^{T} \mathbf{\alpha}^{T})(1- \sigma( \mathbf{\alpha} \mathbf{x}_{i} \mathbf{x}_{i}^{T} \mathbf{\alpha}^{T})) -2(\sigma( \mathbf{\alpha} \mathbf{x}_{i} \mathbf{x}_{i}^{T} \mathbf{\alpha}^{T}))^{2}(1- \sigma( \mathbf{\alpha} \mathbf{x}_{i} \mathbf{x}_{i}^{T} \mathbf{\alpha}^{T}))]4\alpha^{T}\alpha \mathbf{x}_{i}\mathbf{x}^{T}_{i} \nonumber\\ &+ \sigma( \mathbf{\alpha} \mathbf{x}_{i} \mathbf{x}_{i}^{T} \mathbf{\alpha}^{T})(1 - \sigma( \mathbf{\alpha} \mathbf{x}_{i} \mathbf{x}_{i}^{T} \mathbf{\alpha}^{T})) 2\mathbf{x}_{i}\mathbf{x}^{T}_{i} \} \nonumber\\ &- \frac{2}{T^{2}} \sum_{i=1}^{T} \sigma(\mathbf{x}_{i}^{T} \mathbf{\alpha})(1- \sigma(\mathbf{x}_{i}^{T} \mathbf{\alpha}))\sum_{i=1}^{T}\sigma(\mathbf{x}_{i}^{T} \mathbf{\alpha})(1- \sigma(\mathbf{x}_{i}^{T} \mathbf{\alpha})) \nonumber\\ &-\frac{2}{T^{2}}\sum_{i=1}^{T} \sigma(\mathbf{x}_{i}^{T} \mathbf{\alpha}) \sum_{i=1}^{T} [\sigma(\mathbf{x}_{i}^{T} \mathbf{\alpha})(1- \sigma(\mathbf{x}_{i}^{T} \mathbf{\alpha})) -2(\sigma(\mathbf{x}_{i}^{T} \mathbf{\alpha}))^2(1-\sigma(\mathbf{x}_{i}^{T} \mathbf{\alpha}))] \mathbf{x}_{i} \mathbf{x}_{i}^{T} \\ %####################
&= \frac{1}{T} \sum_{i=1}^{T} \{ [\sigma_{x^2}(1- \sigma_{x^2}) -2\sigma_{x^2}^{2}(1- \sigma_{x^2})]4\alpha^{T}\alpha \mathbf{x}_{i}\mathbf{x}^{T}_{i} + \sigma_{x^2}(1 - \sigma_{x^2}) 2\mathbf{x}_{i}\mathbf{x}^{T}_{i} \} \nonumber\\ &- \frac{2}{T^{2}} \sum_{i=1}^{T} \sigma_{x}(1- \sigma_{x})\sum_{i=1}^{T}\sigma_{x}(1- \sigma_{x}) -\frac{2}{T^{2}}\sum_{i=1}^{T} \sigma_{x} \sum_{i=1}^{T} [\sigma_{x}(1- \sigma_{x}) -2(\sigma_{x})^2(1-\sigma_{x})] \mathbf{x}_{i} \mathbf{x}_{i}^{T} \\
% \nabla_{\alpha}^{2} \mathcal{L}_{\text{valid}}^{\text{UDARTS}} &= \frac{1}{N} \sum_{i=1}^{N} \sigma\left(\mathbf{x}_{i}^{T} \mathbf{\alpha}\right)\left(1-\sigma\left(\mathbf{x}_{i}^{T} \mathbf{\alpha}\right)\right) \mathbf{x}_{i} \mathbf{x}_{i}^{T} + \nonumber\\ &\frac{1}{T} \sum_{i=1}^{T} \{ [\sigma( \mathbf{\alpha} \mathbf{x}_{i} \mathbf{x}_{i}^{T} \mathbf{\alpha}^{T})(1- \sigma( \mathbf{\alpha} \mathbf{x}_{i} \mathbf{x}_{i}^{T} \mathbf{\alpha}^{T})) -2(\sigma( \mathbf{\alpha} \mathbf{x}_{i} \mathbf{x}_{i}^{T} \mathbf{\alpha}^{T}))^{2}(1- \sigma( \mathbf{\alpha} \mathbf{x}_{i} \mathbf{x}_{i}^{T} \mathbf{\alpha}^{T}))]4\alpha^{T}\alpha \mathbf{x}_{i}\mathbf{x}^{T}_{i} \nonumber\\ &+ \sigma( \mathbf{\alpha} \mathbf{x}_{i} \mathbf{x}_{i}^{T} \mathbf{\alpha}^{T})(1 - \sigma( \mathbf{\alpha} \mathbf{x}_{i} \mathbf{x}_{i}^{T} \mathbf{\alpha}^{T})) 2\mathbf{x}_{i}\mathbf{x}^{T}_{i} \} \nonumber\\ &- \frac{2}{T^{2}} \sum_{i=1}^{T} \sigma(\mathbf{x}_{i}^{T} \mathbf{\alpha})(1- \sigma(\mathbf{x}_{i}^{T} \mathbf{\alpha}))\sum_{i=1}^{T}\sigma(\mathbf{x}_{i}^{T} \mathbf{\alpha})(1- \sigma(\mathbf{x}_{i}^{T} \mathbf{\alpha})) \nonumber\\ &-\frac{2}{T^{2}}\sum_{i=1}^{T} \sigma(\mathbf{x}_{i}^{T} \mathbf{\alpha}) \sum_{i=1}^{T} [\sigma(\mathbf{x}_{i}^{T} \mathbf{\alpha})(1- \sigma(\mathbf{x}_{i}^{T} \mathbf{\alpha})) -2(\sigma(\mathbf{x}_{i}^{T} \mathbf{\alpha}))^2(1-\sigma(\mathbf{x}_{i}^{T} \mathbf{\alpha}))] \mathbf{x}_{i} \mathbf{x}_{i}^{T}\\ %############################
\nabla_{\alpha}^{2} \mathcal{L}_{\text{valid}}^{\text{UDARTS}} &= \nabla_{\alpha}^{2} \mathcal{L}_{\text{valid}}^{\text{DARTS}} +  \nabla_{\alpha}^{2} \operatorname{Var}_{p(\mathbf{y} | \mathbf{x})}^{model}(\mathbf{\alpha}) \nonumber\\
 &= \frac{1}{N} \sum_{i=1}^{N} \sigma_{x}\left(1-\sigma_{x}\right) \mathbf{x}_{i} \mathbf{x}_{i}^{T} + \nonumber\\ &\frac{1}{T} \sum_{i=1}^{T} \{ [\sigma_{x^2}(1- \sigma_{x^2}) -2\sigma_{x^2}^{2}(1- \sigma_{x^2})]4\alpha^{T}\alpha \mathbf{x}_{i}\mathbf{x}^{T}_{i} + \sigma_{x^2}(1 - \sigma_{x^2}) 2\mathbf{x}_{i}\mathbf{x}^{T}_{i} \} \nonumber\\ &- \frac{2}{T^{2}} \sum_{i=1}^{T} \sigma_{x}(1- \sigma_{x})\sum_{i=1}^{T}\sigma_{x}(1- \sigma_{x}) -\frac{2}{T^{2}}\sum_{i=1}^{T} \sigma_{x} \sum_{i=1}^{T} [\sigma_{x}(1- \sigma_{x}) -2(\sigma_{x})^2(1-\sigma_{x})] \mathbf{x}_{i} \mathbf{x}_{i}^{T}
\end{align}

Since we can choose the number of samples $T$, without loss of generality, let us consider the case when $T=N$.
Again, since the softmax is a convex function, we can use Jensen's inequality as $ \sigma_{x}^{2} \le \sigma_{x^2}$
Also, we note that the maximum value of $\sigma_{x}(1- \sigma_{x})$ is $\frac{1}{4}$, so $\sum_{i=1}^{T} \sigma_{x}(1- \sigma_{x}) \le  \sum_{i=1}^{T} \frac{1}{4} = \frac{T}{4}$. Similarly, the maximum value of $ [\sigma_{x}(1- \sigma_{x}) -2(\sigma_{x})^2(1-\sigma_{x})]$ is given as $0.0962$. Therefore, $\sum_{i=1}^{T} [\sigma_{x}(1- \sigma_{x}) -2(\sigma_{x})^2(1-\sigma_{x})] \le 0.0962T$

Therefore the hessian simplifies to the following form:
\begin{align}
\nabla_{\alpha}^{2} \mathcal{L}_{\text{valid}}^{\text{UDARTS}} 
% &\le  \frac{1}{T} \sum_{i=1}^{T} [\sigma\left(\mathbf{x}_{i}^{T} \mathbf{\alpha}\right)\left(1-\sigma\left(\mathbf{x}_{i}^{T} \mathbf{\alpha}\right)\right)  + \nonumber \\ & \{ [4\sigma( \mathbf{\alpha} \mathbf{x}_{i} \mathbf{x}_{i}^{T} \mathbf{\alpha}^{T})(1- \sigma( \mathbf{\alpha} \mathbf{x}_{i} \mathbf{x}_{i}^{T} \mathbf{\alpha}^{T})) -8(\sigma( \mathbf{\alpha} \mathbf{x}_{i} \mathbf{x}_{i}^{T} \mathbf{\alpha}^{T}))^{2}(1- \sigma( \mathbf{\alpha} \mathbf{x}_{i} \mathbf{x}_{i}^{T} \mathbf{\alpha}^{T}))]\alpha^{T}\alpha \nonumber\\ &+ 2\sigma( \mathbf{\alpha} \mathbf{x}_{i} \mathbf{x}_{i}^{T} \mathbf{\alpha}^{T})(1 - \sigma( \mathbf{\alpha} \mathbf{x}_{i} \mathbf{x}_{i}^{T} \mathbf{\alpha}^{T}))  \} \nonumber\\ &-\frac{1}{2} \sigma(\mathbf{x}_{i}^{T} \mathbf{\alpha})(1- \sigma(\mathbf{x}_{i}^{T} \mathbf{\alpha})) -0.1924 \sigma(\mathbf{x}_{i}^{T} \mathbf{\alpha})] \mathbf{x}_{i} \mathbf{x}_{i}^{T} \\
&\le  \frac{1}{T} \sum_{i=1}^{T} [\sigma_{x}\left(1-\sigma_{x}\right)  + \{ [4\sigma_{x^2}(1- \sigma_{x^2}) -8(\sigma_{x^2})^{2}(1- \sigma_{x^2})]\alpha^{T}\alpha \nonumber\\ &- 2\sigma_{x^2}(1 - \sigma_{x^2})  \} -\frac{1}{2} \sigma_{x}(1- \sigma_{x}) -0.1924 \sigma_{x}] \mathbf{x}_{i} \mathbf{x}_{i}^{T} \\
%  &\le  \frac{1}{T} \sum_{i=1}^{T} [\sqrt{\sigma( \mathbf{\alpha} \mathbf{x}_{i} \mathbf{x}_{i}^{T} \mathbf{\alpha}^{T})}\left(1-\sqrt{\sigma( \mathbf{\alpha} \mathbf{x}_{i} \mathbf{x}_{i}^{T} \mathbf{\alpha}^{T})}\right)  + \nonumber\\ & 4\alpha^2 \sigma( \mathbf{\alpha} \mathbf{x}_{i} \mathbf{x}_{i}^{T} \mathbf{\alpha}^{T})(1- \sigma( \mathbf{\alpha} \mathbf{x}_{i} \mathbf{x}_{i}^{T} \mathbf{\alpha}^{T})) -8\alpha^2(\sigma( \mathbf{\alpha} \mathbf{x}_{i} \mathbf{x}_{i}^{T} \mathbf{\alpha}^{T}))^{2}(1- \sigma( \mathbf{\alpha} \mathbf{x}_{i} \mathbf{x}_{i}^{T} \mathbf{\alpha}^{T}))] \nonumber\\&+ 2\sigma( \mathbf{\alpha} \mathbf{x}_{i} \mathbf{x}_{i}^{T} \mathbf{\alpha}^{T})(1 - \sigma( \mathbf{\alpha} \mathbf{x}_{i} \mathbf{x}_{i}^{T} \mathbf{\alpha}^{T})) \nonumber\\ &-\frac{1}{2}\sqrt{\sigma( \mathbf{\alpha} \mathbf{x}_{i} \mathbf{x}_{i}^{T} \mathbf{\alpha}^{T})}(1 - \sqrt{\sigma( \mathbf{\alpha} \mathbf{x}_{i} \mathbf{x}_{i}^{T} \mathbf{\alpha}^{T})}) -0.1924 \sqrt{\sigma( \mathbf{\alpha} \mathbf{x}_{i} \mathbf{x}_{i}^{T} \mathbf{\alpha}^{T})} ] \mathbf{x}_{i} \mathbf{x}_{i}^{T} \\
 &\le  \frac{1}{T} \sum_{i=1}^{T} [\sqrt{\sigma_{x^2}}\left(1-\sqrt{\sigma_{x^2}}\right)  +  4\alpha^2 \sigma_{x^2}(1- \sigma_{x^2}) -8\alpha^2(\sigma_{x^2})^{2}(1- \sigma_{x^2}) \nonumber\\&- 2\sigma_{x^2}(1 - \sigma_{x^2}) -\frac{1}{2}\sqrt{\sigma_{x^2}}(1 - \sqrt{\sigma_{x^2}}) -0.1924 \sqrt{\sigma_{x^2}} ] \mathbf{x}_{i} \mathbf{x}_{i}^{T} \\
    \Rightarrow \mathbf{z}^{T} \nabla_{\alpha}^{2} \mathcal{L}_{\text{valid}}^{\text{UDARTS}}  \mathbf{z} &\leq \frac{\max \sigma_j}{ N} \mathbf{z}^{T}\left(\sum_{i=1}^{N} \mathbf{x}_{i} \mathbf{x}_{i}^{T}\right) \mathbf{z}
\end{align}

where $\sigma_j = \sqrt{\sigma_{x^2}}\left(1-\sqrt{\sigma_{x^2}}\right)  +  4\alpha^2 \sigma_{x^2}(1- \sigma_{x^2}) -8\alpha^2(\sigma_{x^2})^{2}(1- \sigma_{x^2}) - 2\sigma_{x^2}(1 - \sigma_{x^2}) -\frac{1}{2}\sqrt{\sigma_{x^2}}(1 - \sqrt{\sigma_{x^2}}) -0.1924 \sqrt{\sigma_{x^2}} $

Therefore, the spectral radius of the UDARTS method is given as:
\begin{equation}
\rho(\nabla_{\alpha}^{2}\mathcal{L}_{\text{valid}}^{\text{UDARTS}}) = \frac{\max \sigma_j}{N}\left\|\sum_{i=1}^{N} \mathbf{x}_{i} \mathbf{x}_{i}^{T}\right\|_{2}^{2}
\end{equation}

% We know that the spectral radius of the normal DARTS method is given as 
% \begin{equation}
% \rho(\nabla_{\alpha}^{2}\mathcal{L}_{\text{valid}}^{\text{DARTS}}) = \frac{\max \sigma_{x}\left(1-\sigma_{x}\right)}{ N}\left\|\sum_{i=1}^{N} \mathbf{x}_{i} \mathbf{x}_{i}^{T}\right\|_{2}^{2}.
% \end{equation}
So, now to show that the spectral radius of the UDARTS method is smaller than that of the general DARTS method, we need to only show that $\max \sigma_j \le \max \sigma_i$.
Treating this equation as a polynomial in $\sigma_{x^2}$ such that the values of $\sigma(\mathbf{x}_{i}^{T} \mathbf{\alpha}) \in [0,1]$, we get the following polynomial: $\sigma_j = \frac{1}{2} \sqrt{x}(1-\sqrt{x})+4\alpha^2[ x(1-x)- 2x^{2}(1-x)]-2 x(1-x)-0.1924 \sqrt{x}$. Now, since sigmoid function $\sigma$ is represented as $x$, the domain of our function is $[0,1]$. Thus, the maximum value of the polynomial is  achieved at $x= 0.1132$ when it reached the value $(0.310634)\alpha^2 -0.15388$> Thus, we can see that $\max \sigma_j \le \sigma_i$ for $\alpha^2 < 1.3$.  Since $\alpha$ is the weights in the neural network, $\alpha < 1 \Rightarrow \alpha^2 < 1$. Hence, the maximum value of the function is always lesser than the maximum value of the standard DARTS method.

Hence we may say that the spectral radius of the hessian of the UDARTS are smaller than the ones of the DARTS method. Therefore, 
\[\rho(\nabla_{\alpha}^{2}\mathcal{L}_{\text{valid}}^{\text{DARTS}})  \ge \rho(\nabla_{\alpha}^{2}\mathcal{L}_{\text{valid}}^{\text{UDARTS}})  \]

% \subsection*{Spectral radius of the Architecture}
