# Supplementary material for: $\mu$DARTS: Model Uncertainty-Aware Differentiable Architecture Search
Source: arXiv:2107.11500 source file (2022-09-11)
Supplement: Supplementary file 2 [file Appendix1.tex]

\section*{Appendix A}

\subsection*{Comparison of spectral radius of DARTS vs UDARTS}

\textbf{Proof: }

We aim to prove that the inclusion of the predictive variance improves the performance of the UDARTS method compared to normal DARTS and will search for a flatter minima.
In order to prove this, we aim to show that the spectral radius of the Hessian of the validation loss $\rho(\nabla_{\alpha}^2 \mathcal{L}_{\text{valid}})$ is smaller than the spectral radius of the normal DARTS method.  First of all we consider the cross entropy loss which is used to calculate the basic validation loss $\mathcal{L}_{\text{valid}}$. 
The gradient and the corresponding hessian of the cross entropy loss are given as follows:
\begin{equation}g(\mathbf{\alpha})=-\frac{1}{N} \sum_{i=1}^{N} y_{i} \log \left(\sigma\left(\operatorname{model}\left(\mathbf{x}_{i}, \mathbf{\alpha}\right)\right)\right)+\left(1-y_{i}\right) \log \left(1-\sigma\left(\operatorname{model}\left(\mathbf{x}_{i}, \mathbf{\alpha}\right)\right)\right)\end{equation}

For this proof we consider a linear model given as $\operatorname{model}\left(\mathbf{x}_{i}, \mathbf{\alpha}\right)=\mathbf{x}_{i}^{T} \mathbf{\alpha}$

\begin{equation}\nabla_{\alpha} g(\mathbf{\alpha})=-\frac{1}{N} \sum_{i=1}^{N}\left(y_{i}-\sigma\left(\mathbf{x}_{i}^{T} \mathbf{\alpha}\right)\right) \mathbf{x}_{i}\end{equation}

\begin{equation}\nabla_{\alpha}^{2} g(\mathbf{\alpha})=\frac{1}{N} \sum_{i=1}^{N} \sigma\left(\mathbf{x}_{i}^{T} \mathbf{\alpha}\right)\left(1-\sigma\left(\mathbf{x}_{i}^{T} \mathbf{\alpha}\right)\right) \mathbf{x}_{i} \mathbf{x}_{i}^{T}\end{equation}

Now, in order to prove that the cross entropy function is convex, we prove that the hessian is positive semi-definite. We know that the smallest eigenvalue of any square symmetric matrix is given as the minimum of the Rayleigh quotient, i.e., the smallest value taken by

\[
\mathbf{z}^{T} \nabla_{\alpha}^{2} g(\mathbf{\alpha}) \mathbf{z}
\]
for any unit-length vector $\mathbf{z}$ and any possible weight vector $\mathbf{\alpha}$. Substituting in the particular form of the Hessian here, denoting $\sigma_{i}=\sigma\left(\mathbf{x}_{i}^{T} \mathbf{\alpha}\right)\left(1-\sigma\left(\mathbf{x}_{i}^{T} \mathbf{\alpha}\right)\right)$ for each $i$ for short, we have
\begin{equation}
\mathbf{z}^{T} \nabla_{\alpha}^{2} g(\mathbf{\alpha}) \mathbf{z}=\mathbf{z}^{T}\left(\frac{1}{N} \sum_{i=1}^{N} \sigma_{i} \mathbf{x}_{i} \mathbf{x}_{i}^{T}\right) \mathbf{z}=\frac{1}{N} \sum_{i=1}^{N} \sigma_{i}\left(\mathbf{z}^{T} \mathbf{x}_{i}\right)\left(\mathbf{x}_{i}^{T} \mathbf{z}\right)=\frac{1}{N} \sum_{i=1}^{N} \sigma_{i}\left(\mathbf{z}^{T} \mathbf{x}_{i}\right)^{2}
\end{equation}
since it is always the case that $\left(\mathbf{z}^{T} \mathbf{x}_{i}\right)^{2} \geq 0$ and $\sigma_{i} \geq 0,$ it follows that the smallest value the above can take is 0 meaning that this is the smallest possible eigenvalue of the softmax cost's Hessian. since this is the case, the softmax
cost must be convex.
We know that for a matrix $A$, 
\begin{equation}\|A\|_{2}^{2}=\max _{x \neq 0} \frac{\|A x\|_{2}^{2}}{\|x\|_{2}^{2}}=\max _{x \neq 0} \frac{x^{T} A^{T} A x}{x^{T} x}=\lambda_{\max }\left(A^{T} A\right)=\rho\left(A^{T} A\right)\end{equation}

Building on the analysis above showing that the cross-entropy cost is convex, we can likewise compute its largest possible eigenvalue by noting that $\sigma_{i} \le \frac{1}{4}$. Thus the largest value the Rayleigh quotient can take is bounded above for any $\mathbf{z}$ as
\[
\mathbf{z}^{T} \nabla_{\alpha}^{2} g(\mathbf{\alpha}) \mathbf{z} \leq \frac{1}{4 N} \mathbf{z}^{T}\left(\sum_{i=1}^{N} \mathbf{x}_{i} \mathbf{x}_{i}^{T}\right) \mathbf{z}
\]
since the maximum value $\mathbf{z}^{T}\left(\sum_{i=1}^{N} \mathbf{x}_{i} \mathbf{x}_{i}^{T}\right) \mathbf{z}$ can take is the maximum eigenvalue of the matrix $\sum_{i=1}^{N} \mathbf{x}_{i} \mathbf{x}_{i}^{T},$ thus the spectral radius for the Cross Entropy cost is given as
\[
\rho(\nabla_{\alpha}^{2}\mathcal{L}_{\text{valid}}^{\text{DARTS}}) = \frac{1}{4 N}\left\|\sum_{i=1}^{N} \mathbf{x}_{i} \mathbf{x}_{i}^{T}\right\|_{2}^{2}
\]

Now for the case of UDARTS, we add the predictive variance term to the DARTS validation loss.

\begin{align}
\operatorname{Var}_{p(\mathbf{y} | \mathbf{x})}^{model}(\mathbf{\alpha})
&= \frac{1}{T} \sum_{i=1}^{T}\sigma( \mathbf{\alpha} \mathbf{x}_{i} \mathbf{x}_{i}^{T} \mathbf{\alpha}^{T}) - \frac{1}{T}( \sum_{i=1}^{T}\sigma(\mathbf{x}_{i}^{T} \mathbf{\alpha}))^{2}\\
\nabla_{\alpha} \operatorname{Var}_{p(\mathbf{y} | \mathbf{x})}^{model}(\mathbf{\alpha}) &= \frac{1}{T} \sum_{i=1}^{T}\sigma(\mathbf{\alpha} \mathbf{x}_{i} \mathbf{x}_{i}^{T} \mathbf{\alpha}^{T})(1- \sigma(\mathbf{\alpha} \mathbf{x}_{i} \mathbf{x}_{i}^{T} \mathbf{\alpha}^{T})) 2\mathbf{\alpha}^{T}\mathbf{x}_{i} -  \frac{2}{T^{2}} \sum_{i=1}^{T} \sigma(\mathbf{x}_{i}^{T} \mathbf{\alpha}) \sum_{i=1}^{T} \sigma(\mathbf{x}_{i}^{T} \mathbf{\alpha}) (1 - \sigma(\mathbf{x}_{i}^{T} \mathbf{\alpha})) \mathbf{x}_{i}\\
\nabla_{\alpha}^{2} \operatorname{Var}_{p(\mathbf{y} | \mathbf{x})}^{model}(\mathbf{\alpha}) &= \frac{1}{T} \sum_{i=1}^{T} \{ [\sigma( \mathbf{\alpha} \mathbf{x}_{i} \mathbf{x}_{i}^{T} \mathbf{\alpha}^{T})(1- \sigma( \mathbf{\alpha} \mathbf{x}_{i} \mathbf{x}_{i}^{T} \mathbf{\alpha}^{T})) -2(\sigma( \mathbf{\alpha} \mathbf{x}_{i} \mathbf{x}_{i}^{T} \mathbf{\alpha}^{T}))^{2}(1- \sigma( \mathbf{\alpha} \mathbf{x}_{i} \mathbf{x}_{i}^{T} \mathbf{\alpha}^{T}))]4\alpha^{T}\alpha \mathbf{x}_{i}\mathbf{x}^{T}_{i} \nonumber\\ &+ \sigma( \mathbf{\alpha} \mathbf{x}_{i} \mathbf{x}_{i}^{T} \mathbf{\alpha}^{T})(1 - \sigma( \mathbf{\alpha} \mathbf{x}_{i} \mathbf{x}_{i}^{T} \mathbf{\alpha}^{T})) 2\mathbf{x}_{i}\mathbf{x}^{T}_{i} \} \nonumber\\ &- \frac{2}{T^{2}} \sum_{i=1}^{T} \sigma(\mathbf{x}_{i}^{T} \mathbf{\alpha})(1- \sigma(\mathbf{x}_{i}^{T} \mathbf{\alpha}))\sum_{i=1}^{T}\sigma(\mathbf{x}_{i}^{T} \mathbf{\alpha})(1- \sigma(\mathbf{x}_{i}^{T} \mathbf{\alpha})) \nonumber\\ &-\frac{2}{T^{2}}\sum_{i=1}^{T} \sigma(\mathbf{x}_{i}^{T} \mathbf{\alpha}) \sum_{i=1}^{T} [\sigma(\mathbf{x}_{i}^{T} \mathbf{\alpha})(1- \sigma(\mathbf{x}_{i}^{T} \mathbf{\alpha})) -2(\sigma(\mathbf{x}_{i}^{T} \mathbf{\alpha}))^2(1-\sigma(\mathbf{x}_{i}^{T} \mathbf{\alpha}))] \mathbf{x}_{i} \mathbf{x}_{i}^{T} \\
% &= \frac{1}{T} \sum_{i=1}^{T}\sigma(\mathbf{x}_{i}^{T} \mathbf{\alpha})(1- \sigma(\mathbf{x}_{i}^{T} \mathbf{\alpha}))[1- 2\sigma(\mathbf{x}_{i}^{T} \mathbf{\alpha})]\mathbf{x}_{i}\mathbf{x}_{i}^{T} \\
\nabla_{\alpha}^{2} \mathcal{L}_{\text{valid}}^{\text{UDARTS}} &= \frac{1}{N} \sum_{i=1}^{N} \sigma\left(\mathbf{x}_{i}^{T} \mathbf{\alpha}\right)\left(1-\sigma\left(\mathbf{x}_{i}^{T} \mathbf{\alpha}\right)\right) \mathbf{x}_{i} \mathbf{x}_{i}^{T} + \nonumber\\ &\frac{1}{T} \sum_{i=1}^{T} \{ [\sigma( \mathbf{\alpha} \mathbf{x}_{i} \mathbf{x}_{i}^{T} \mathbf{\alpha}^{T})(1- \sigma( \mathbf{\alpha} \mathbf{x}_{i} \mathbf{x}_{i}^{T} \mathbf{\alpha}^{T})) -2(\sigma( \mathbf{\alpha} \mathbf{x}_{i} \mathbf{x}_{i}^{T} \mathbf{\alpha}^{T}))^{2}(1- \sigma( \mathbf{\alpha} \mathbf{x}_{i} \mathbf{x}_{i}^{T} \mathbf{\alpha}^{T}))]4\alpha^{T}\alpha \mathbf{x}_{i}\mathbf{x}^{T}_{i} \nonumber\\ &+ \sigma( \mathbf{\alpha} \mathbf{x}_{i} \mathbf{x}_{i}^{T} \mathbf{\alpha}^{T})(1 - \sigma( \mathbf{\alpha} \mathbf{x}_{i} \mathbf{x}_{i}^{T} \mathbf{\alpha}^{T})) 2\mathbf{x}_{i}\mathbf{x}^{T}_{i} \} \nonumber\\ &- \frac{2}{T^{2}} \sum_{i=1}^{T} \sigma(\mathbf{x}_{i}^{T} \mathbf{\alpha})(1- \sigma(\mathbf{x}_{i}^{T} \mathbf{\alpha}))\sum_{i=1}^{T}\sigma(\mathbf{x}_{i}^{T} \mathbf{\alpha})(1- \sigma(\mathbf{x}_{i}^{T} \mathbf{\alpha})) \nonumber\\ &-\frac{2}{T^{2}}\sum_{i=1}^{T} \sigma(\mathbf{x}_{i}^{T} \mathbf{\alpha}) \sum_{i=1}^{T} [\sigma(\mathbf{x}_{i}^{T} \mathbf{\alpha})(1- \sigma(\mathbf{x}_{i}^{T} \mathbf{\alpha})) -2(\sigma(\mathbf{x}_{i}^{T} \mathbf{\alpha}))^2(1-\sigma(\mathbf{x}_{i}^{T} \mathbf{\alpha}))] \mathbf{x}_{i} \mathbf{x}_{i}^{T}
\end{align}

Since we can choose the number of samples $T$, without loss of generality, let us consider the case when $T=N$.
Again, since the softmax is a convex function, we can use Jensen's inequality as \[ (\sigma\left(\mathbf{x}_{i}^{T} \mathbf{\alpha}\right))^{2} \le \sigma( \mathbf{\alpha} \mathbf{x}_{i} \mathbf{x}_{i}^{T} \mathbf{\alpha}^{T})\]. Also, we note that the maximum value of $\sigma(\mathbf{x}_{i}^{T} \mathbf{\alpha})(1- \sigma(\mathbf{x}_{i}^{T} \mathbf{\alpha}))$ is $\frac{1}{4}$, so $\sum_{i=1}^{T} \sigma(\mathbf{x}_{i}^{T} \mathbf{\alpha})(1- \sigma(\mathbf{x}_{i}^{T} \mathbf{\alpha})) \le  \sum_{i=1}^{T} \frac{1}{4} = \frac{T}{4}$. Similarly, the maximum value of $ [\sigma(\mathbf{x}_{i}^{T} \mathbf{\alpha})(1- \sigma(\mathbf{x}_{i}^{T} \mathbf{\alpha})) -2(\sigma(\mathbf{x}_{i}^{T} \mathbf{\alpha}))^2(1-\sigma(\mathbf{x}_{i}^{T} \mathbf{\alpha}))]$ is given as $0.0962$. Therefore, $\sum_{i=1}^{T} [\sigma(\mathbf{x}_{i}^{T} \mathbf{\alpha})(1- \sigma(\mathbf{x}_{i}^{T} \mathbf{\alpha})) -2(\sigma(\mathbf{x}_{i}^{T} \mathbf{\alpha}))^2(1-\sigma(\mathbf{x}_{i}^{T} \mathbf{\alpha}))] \le 0.0962T$

Therefore the hessian simplifies to the following form:
\begin{align}
\nabla_{\alpha}^{2} \mathcal{L}_{\text{valid}}^{\text{UDARTS}} &\le  \frac{1}{T} \sum_{i=1}^{T} [\sigma\left(\mathbf{x}_{i}^{T} \mathbf{\alpha}\right)\left(1-\sigma\left(\mathbf{x}_{i}^{T} \mathbf{\alpha}\right)\right)  + \nonumber \\ & \{ [4\sigma( \mathbf{\alpha} \mathbf{x}_{i} \mathbf{x}_{i}^{T} \mathbf{\alpha}^{T})(1- \sigma( \mathbf{\alpha} \mathbf{x}_{i} \mathbf{x}_{i}^{T} \mathbf{\alpha}^{T})) -8(\sigma( \mathbf{\alpha} \mathbf{x}_{i} \mathbf{x}_{i}^{T} \mathbf{\alpha}^{T}))^{2}(1- \sigma( \mathbf{\alpha} \mathbf{x}_{i} \mathbf{x}_{i}^{T} \mathbf{\alpha}^{T}))]\alpha^{T}\alpha \nonumber\\ &+ 2\sigma( \mathbf{\alpha} \mathbf{x}_{i} \mathbf{x}_{i}^{T} \mathbf{\alpha}^{T})(1 - \sigma( \mathbf{\alpha} \mathbf{x}_{i} \mathbf{x}_{i}^{T} \mathbf{\alpha}^{T}))  \} \nonumber\\ &-\frac{1}{2} \sigma(\mathbf{x}_{i}^{T} \mathbf{\alpha})(1- \sigma(\mathbf{x}_{i}^{T} \mathbf{\alpha})) -0.1924 \sigma(\mathbf{x}_{i}^{T} \mathbf{\alpha})] \mathbf{x}_{i} \mathbf{x}_{i}^{T} \\
 &\le  \frac{1}{T} \sum_{i=1}^{T} [\sqrt{\sigma( \mathbf{\alpha} \mathbf{x}_{i} \mathbf{x}_{i}^{T} \mathbf{\alpha}^{T})}\left(1-\sqrt{\sigma( \mathbf{\alpha} \mathbf{x}_{i} \mathbf{x}_{i}^{T} \mathbf{\alpha}^{T})}\right)  + \nonumber\\ & 4\alpha^2 \sigma( \mathbf{\alpha} \mathbf{x}_{i} \mathbf{x}_{i}^{T} \mathbf{\alpha}^{T})(1- \sigma( \mathbf{\alpha} \mathbf{x}_{i} \mathbf{x}_{i}^{T} \mathbf{\alpha}^{T})) -8\alpha^2(\sigma( \mathbf{\alpha} \mathbf{x}_{i} \mathbf{x}_{i}^{T} \mathbf{\alpha}^{T}))^{2}(1- \sigma( \mathbf{\alpha} \mathbf{x}_{i} \mathbf{x}_{i}^{T} \mathbf{\alpha}^{T}))] \nonumber\\&+ 2\sigma( \mathbf{\alpha} \mathbf{x}_{i} \mathbf{x}_{i}^{T} \mathbf{\alpha}^{T})(1 - \sigma( \mathbf{\alpha} \mathbf{x}_{i} \mathbf{x}_{i}^{T} \mathbf{\alpha}^{T})) \nonumber\\ &-\frac{1}{2}\sqrt{\sigma( \mathbf{\alpha} \mathbf{x}_{i} \mathbf{x}_{i}^{T} \mathbf{\alpha}^{T})}(1 - \sqrt{\sigma( \mathbf{\alpha} \mathbf{x}_{i} \mathbf{x}_{i}^{T} \mathbf{\alpha}^{T})}) -0.1924 \sqrt{\sigma( \mathbf{\alpha} \mathbf{x}_{i} \mathbf{x}_{i}^{T} \mathbf{\alpha}^{T})} ] \mathbf{x}_{i} \mathbf{x}_{i}^{T} 
\end{align}

Treating this equation as a polynomial in $\sigma(\mathbf{x}_{i}^{T} \mathbf{\alpha})$ such that the values of $\sigma(\mathbf{x}_{i}^{T} \mathbf{\alpha}) \in [0,1]$, we get the following polynomial: $f(x) = \frac{1}{2} \sqrt{x}(1-\sqrt{x})+4\alpha^2[ x(1-x)- 2x^{2}(1-x)]+2 x(1-x)-0.1924 \sqrt{x}$ such that $\max f(x) \le \max x(1-x)$ for $x \in [0,1]$ since $\alpha^2 < 1$. Hence we may say that the spectral radius of the hessian of the UDARTS are smaller than the ones of the DARTS method

% \subsection*{Spectral radius of the Architecture}
